# Supplementary material for: StyleGAN of All Trades: Image Manipulation with Only Pretrained StyleGAN
Source: arXiv:2111.01619 source file (2021-11-02)
Supplement: Supplementary file 7 [file supp_single_im.tex]

\begin{figure}[t]
    \centering
    \includegraphics[width=1\linewidth]{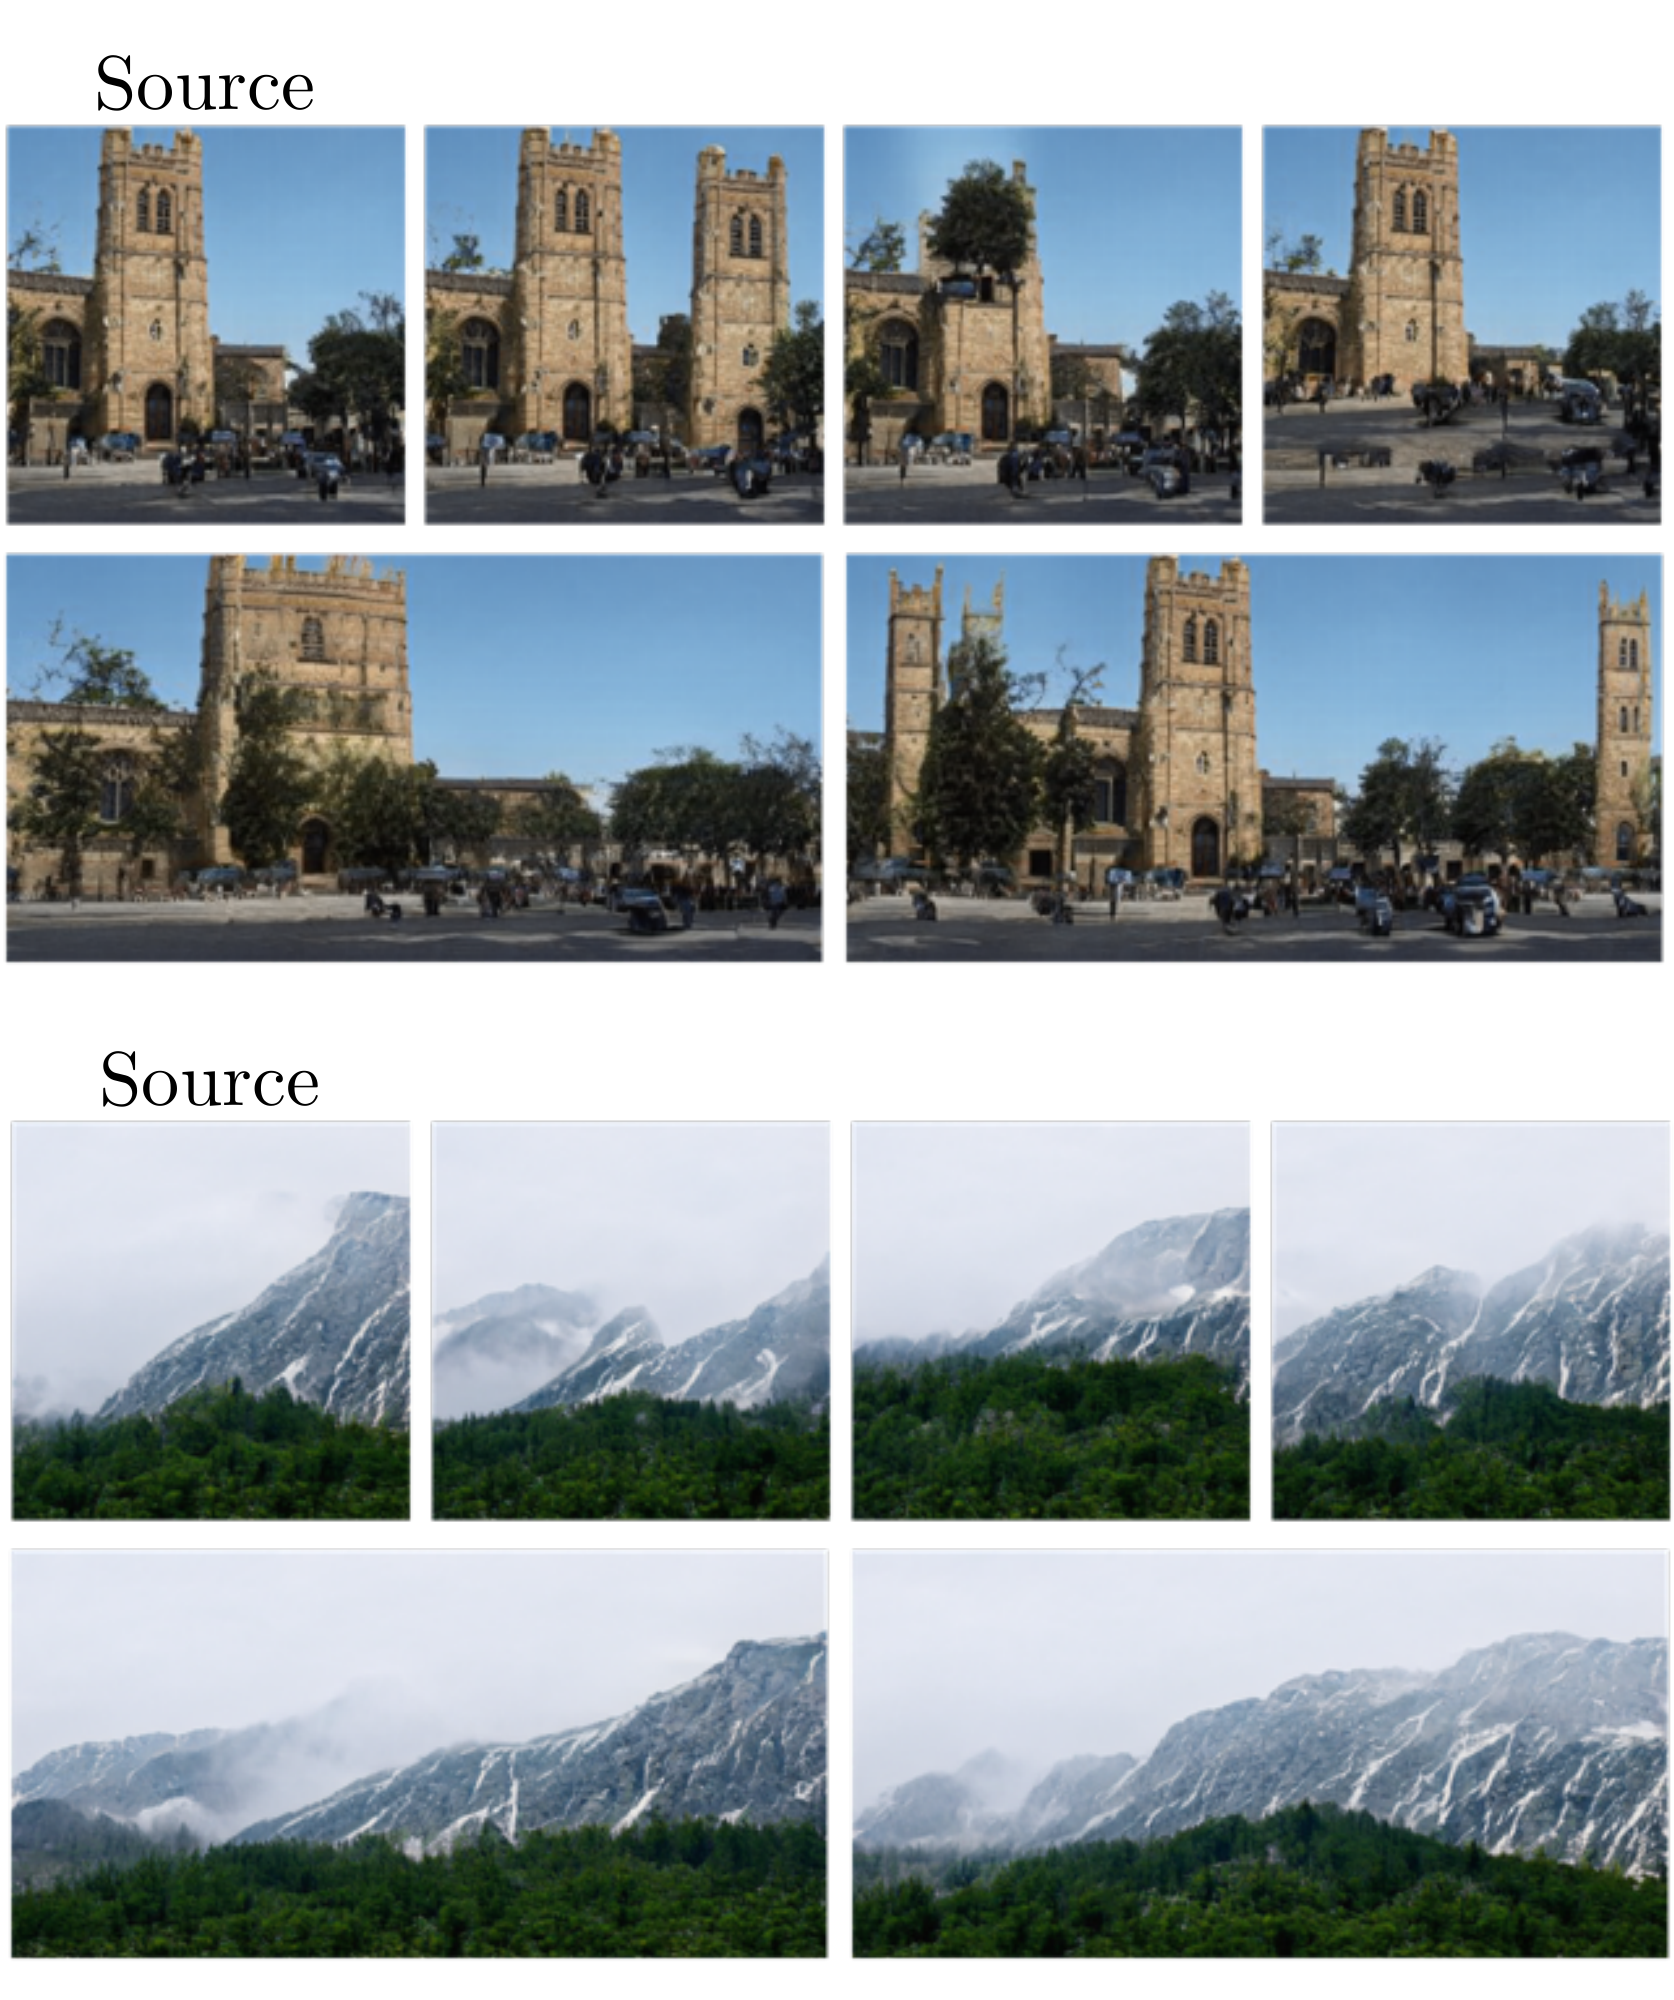}
    \caption{\textbf{More Samples of Generation from a single image.}
    }
    \vspace{\figmargin}
    \label{fig:supp_single_im}
\end{figure}
